# Supplementary material for: Selectively-Amortized Resource Bounding (Extended Version)
Source: arXiv:2108.08263 source file (2021-10-13)
Supplement: Supplementary file 1 [file 09-appendix-old.tex]

\section{OLD: Proof: Soundness of Selectively-Amortized Bounding}

In this section, we prove the soundness of using selectively-amortization decomposition to approximate resource usage, which is stated as \autoref{thm:soundness} in \autoref{sec:resetting-soundness}.

\subsection{Sound Approximation of Resource Usage for Commands}

We prove part \ref{soundness-cmds} in \autoref{thm:soundness}, which we restate as \autoref{thm:sound-cmd}.
\begin{lemma}
  If $\hypdecomp{\orig\cmd}{\cmd}$,
      $\evalcmd{\pstore}{\cmd}{\pstore'}$, and
      $\samevarstore{\orig\pstore}{\pstore}$,
      then $\evalcmd{\orig\pstore}{\orig\cmd}{\orig{\pstore'}}$
      with $\samevarstore{\orig{\pstore'}}{\pstore'}$.
      %\label{thm:sound-cmd}
\end{lemma}

\input{proof-cmd.tex}

\begin{proof}
We first prove there exists a store $\orig{\pstore'}$ such that $\evalcmd{\orig\pstore}{\orig\cmd}{\orig{\pstore'}}$ via \autoref{fig:sound-cmd-1} (Part 1).
Next we prove $\samevarstore{\orig{\pstore'}}{\pstore'}$ by case splitting on the forms of resource-decomposed commands that are defined in \autoref{fig:decomp}, via \autoref{fig:sound-cmd-2} when resource-decomposed commands $\hypdecomp{\orig\cmd}{\cmd}$ is \TirName{D-UBCheck} or \TirName{D-Use} (Part 2.1) and \autoref{fig:sound-cmd-3} when resource-decomposed commands $\hypdecomp{\orig\cmd}{\cmd}$ is \TirName{D-Reset} or \TirName{D-Command} (Part 2.2).
The proof is now complete.\qed
\end{proof}





\subsection{Sound Approximation of Resource Usage for Paths}

We prove part \ref{soundness-paths} in \autoref{thm:soundness}, which we restate as \autoref{thm:sound-path}.
\begin{lemma}
  If $\hypdecomp{\orig\ptrace}{\ptrace}$ and $\ptraceok{\ptrace}$,
      then $\ptraceok{\orig\ptrace}$.
      %\label{thm:sound-path}
\end{lemma}

\input{proof-path.tex}

\begin{proof}
To prove this theorem, we case split on the forms of trace $\ptrace$ defined by \TirName{Ok-Init} and \TirName{Ok-Step}.

First, a trace may be in the of form of $\pstate$ for some $\pstate$.
Since $\hypdecomp{\orig\ptrace}{\ptrace}$, we can only use rule \TirName{D-Init} and thus we have $\ptrace = \pstate$ and $\orig\ptrace = \pstate$.
Since it is assumed (in \autoref{thm:sound-path}) that $\ptraceok{\pstate}$, we have $\ptraceok{\orig\ptrace}$.

Second, a trace may be in the form of $\traceconsstate{\traceconscmd{\ptrace}{\pstore}{\cmd}}{\pstate_\diamond}$ for some $\ptrace, \pstore, \cmd, \pstate_\diamond$.
We prove by induction on the trace.
The steps are (\autoref{fig:sound-path}):
\begin{itemize}
  \item[\textcircled{1}] Since $\hypdecomp{\orig\ptrace}{\traceconsstate{\traceconscmd{\ptrace}{\pstore}{\cmd}}{\pstate_\diamond}}$ and $\ptraceok{\traceconsstate{\traceconscmd{\ptrace}{\pstore}{\cmd}}{\pstate_\diamond}}$, Rule \TirName{D-Step} must be used to derive this conclusion.
  Thus, $\orig\ptrace$ must be $\traceconsstate{\ptrace_\star}{\pstate_\star}$ for some $\ptrace_\star, \pstate_\star$.
   
  \item[\textcircled{2}] To derive the conclusion of $\hypdecomp{\ptrace_\star}{\traceconscmd{\ptrace}{\pstore}{\cmd}}$, according to Rule \TirName{D-AppendCommand} $\ptrace_\star$ must be $\traceconscmd{\ptrace_\vartriangle}{\pstore_\vartriangle}{\cmd_\vartriangle}$ for some \emph{not-yet-determined} $\ptrace_\vartriangle, \pstore_\vartriangle, \cmd_\vartriangle$, as long as they satisfy the constraints in the premises in \textcircled{2}.
   
  \item[\textcircled{3}] The goal is to prove $\ptraceok{\traceconsstate{\traceconscmd{\ptrace_\vartriangle}{\pstore_\vartriangle}{\cmd_\vartriangle}}{\pstate_\star}}$, which can be implied by $\traceconsstate{\ptrace_\vartriangle}{\locstore{\loc_\star}{\pstore_\vartriangle}}$ and $\evalcmd{\pstore_\vartriangle}{\cmd_\vartriangle}{\pstore_\star}$ where $\pstate_\star = \locstore{\loc_\star}{\pstore_\star}$, according to Rule \TirName{Ok-Step}.
  Hence, the goal now is to prove $\ptraceok{\traceconsstate{\ptrace_\vartriangle}{\locstore{\loc_\star}{\pstore_\vartriangle}}}$ and $\evalcmd{\pstore_\vartriangle}{\cmd_\vartriangle}{\pstore_\star}$.
  
  \item[\textcircled{4}] To derive the conclusion of $\hypdecomp{\traceconsstate{\ptrace_\vartriangle}{\locstore{\loc_\vartriangle}{\pstore_\vartriangle}}}{\traceconsstate{\ptrace}{\locstore{\loc}{\pstore}}}$, Rule \TirName{D-Step} must be applied.

  \item[\textcircled{5}] We have $\samevarstore{\pstore_\vartriangle'}{\pstore_\diamond}$ because the assumptions in \autoref{thm:sound-cmd} are satisfied:
  \begin{inparaenum}[(1)]
    \item $\hypdecomp{\cmd_\vartriangle}{\cmd}$,
    \item $\evalcmd{\pstore_\vartriangle}{\cmd_\vartriangle}{\pstore_\vartriangle'}$ for some $\pstore_\vartriangle'$,
    \item $\evalcmd{\pstore}{\cmd}{\pstore_\diamond}$ where $\pstate_\diamond = \locstore{\_}{\pstore_\diamond}$,
    \item $\samevarstore{\pstore_\vartriangle}{\pstore}$.
  \end{inparaenum}

  Now let $\pstore_\vartriangle'$ be $\pstore_\star$, which is always possible due to not violating any facts in \textcircled{1} or \textcircled{2}, especially not violating $\samevarstore{\pstate_\star}{\pstate_\diamond}$.
  Thus, we have proved $\evalcmd{\pstore_\vartriangle}{\cmd_\vartriangle}{\pstore_\star}$.

  \item[\textcircled{6}] We have $\ptraceok{\traceconsstate{\ptrace_\vartriangle}{\locstore{\loc_\vartriangle}{\pstore_\vartriangle}}}$ by the inductive assumption, since the assumptions in \autoref{thm:sound-path} are satisfied in \textcircled{4}:
  \begin{inparaenum}[(1)]
    \item $\hypdecomp{
      \traceconsstate{\ptrace_\vartriangle}{\locstore{\loc_\vartriangle}{\pstore_\vartriangle}}
    }{
      \traceconsstate{\ptrace}{\locstore{\loc}{\pstore}}
    }$,
    \item $\ptraceok{\traceconsstate{\ptrace}{\locstore{\loc}{\pstore}}}$.
  \end{inparaenum}
  Now let $\loc_\vartriangle$ be $\loc_\star$.
  Thus, we have proved $\ptraceok{\traceconsstate{\ptrace_\vartriangle}{\locstore{\loc_\star}{\pstore_\vartriangle}}}$.
\end{itemize}

The proof is now complete.\qed
\end{proof}





\subsection{Sound Approximation of Resource Usage for Programs}

We prove part \ref{soundness-programs} in \autoref{thm:soundness}, which we restate as \autoref{thm:sound-prog}.
\begin{lemma}
  If $\hypdecomp{\orig\prog}{\prog}$
      and $\ptrace \in \denote{\prog} \pstate$,
      then there is a $\orig\ptrace \in \denote{\orig\prog} \pstate$
      s.t. $\hypdecomp{\orig\ptrace}{\ptrace}$.
  %\label{thm:sound-prog}
\end{lemma}

\input{proof-prog.tex}

\begin{proof}
To prove \autoref{thm:sound-prog}, we prove \autoref{lemma:sound-prog}, whose validity directly implies the validity of \autoref{thm:sound-prog}.
\begin{lemma}
  If $\hypdecomp{\orig\prog}{\prog}$, for any $\pstate_0$, consider two paths that both begin with $\pstate_0$ and are executed along a same sequence of locations from $\orig\prog$ and $\prog$: $\traceconsstate{\orig\ptrace}{\orig\pstate}, \traceconsstate{\ptrace}{\pstate}$.
  Then $\hypdecomp{\traceconsstate{\orig\ptrace}{\orig\pstate}}{\traceconsstate{\ptrace}{\pstate}}$ and $\ptraceok{\traceconsstate{\ptrace}{\pstate}}$ where $\orig\pstate = \locstore{\orig\loc}{\orig\pstore}, \pstate = \locstore{\loc}{\pstore}$.
  \label{lemma:sound-prog}
\end{lemma}

We prove \autoref{lemma:sound-prog} by induction on paths.
In the base case, we have $\hypdecomp{\pstate_0}{\pstate_0}$ and $\ptraceok{\pstate_0}$.
In the inductive case, let the current location be $\orig\loc = \loc$ and the next location be $\orig\loc' = \loc'$, because the two paths are executed along a same sequence of locations.
The inductive assumption is:
$\hypdecomp{\traceconsstate{\orig\ptrace}{\orig\pstate}}{\traceconsstate{\ptrace}{\pstate}}$ and $\ptraceok{\traceconsstate{\ptrace}{\pstate}}$ where $\orig\pstate = \locstore{\orig\loc}{\orig\pstore}, \pstate = \locstore{\loc}{\pstore}$.
Then the inductive case can be proven by the derivation tree in \autoref{fig:sound-prog-1} and \autoref{fig:sound-prog-2}, where the premises in the leaf inference rules are either induction assumptions or facts.
The proof is now complete.\qed
\end{proof}
